# Supplementary material for: Accurate Performance Modeling And Uncertainty Analysis of Lossy Compression in Scientific Applications
Source: arXiv:2412.07015 source file (2024-12-09)
Supplement: Supplementary file 1 [file 09_appendix.tex]

% \newpage

\appendix
